# Supplementary material for: Strategic investments in multi-stage General Lotto games
Source: arXiv:2209.06090 source file (2022-09-13)
Supplement: Supplementary file 1 [file appendix.tex]

% % % % % % % % % % % % % % % %
% % % % OLD PROOF % % % %
% % % % % % % % % % % % % % % %

% \begin{lemma}\label{lem:piA_unif_cost}
%     For any $S \in [0,X_A/c]$ (with $M_A = X_A - cS$), the payoff $\pi_A(S,X_A-cS,M_B)$ to player $A$ is given as follows. If either of the following three conditions hold:
%     \begin{enumerate}
%         \item $S \in [0,S_-]$ and $S_- \in (0,X_A/c)$, or
%         \item $S \in [S_+,\min\{qM_B,X_A/c\}]$ and $S_+ \leq \min\{qM_B,X_A/c\}$, or
%         \item $X_A \leq 2qM_B(2-c)\left(\sqrt{1 + \frac{c}{2-c}} - 1 \right)$
%     \end{enumerate}
%     where $S_\pm := qM_B - \frac{X_A}{2(2-c)} \pm \sqrt{\frac{qM_B(X_A-cqM_B)}{2-c} + \left(\frac{X_A}{2(2-c)} \right)^2}$, then
%     \begin{equation}\label{eq:piA3_cost}
%         \pi_A(S,X_A-cS,M_B) = W\cdot \frac{X_A-cS}{2(qM_B - S)}.
%     \end{equation}
%     If none of the above three conditions hold, then $\pi_A(S,X_A-cS,M_B)$ is given by
%     \begin{equation}\label{eq:piA2_cost}
%         W\cdot\left(1 - \frac{qM_B}{2}\left(\frac{\sqrt{M_A} + \sqrt{M_A+2S}}{\sqrt{M_A}(\sqrt{M_A} + \sqrt{M_A+2S}) + S} \right)^2 \right).
%     \end{equation}
% \end{lemma}
% \begin{proof}
%     Our approach is to first explicitly derive $\pi_A(S,M_A,M_B)$ using Lemma \ref{lem:SOE} for arbitrary $S,M_A,M_B > 0$. We then substitute $M_A = X_A-cS$ for any $S \leq \frac{X_A}{c}$ into this characterization to prove the result.
    
%     % {\color{red}
%     % Using Fact \ref{fact:SOE} and the conditions derived for Case 1 and 2, the equilibrium payoff $\pi_A(S,M_A,M_B)$ to player $A$ is given by 
%     % \begin{equation}
%     %     nw\cdot
%     %     \begin{cases}
%     %         1 - \frac{qM_B}{2M_A}\left(\frac{M_A + \sqrt{M_A(M_A+2S)}}{S+M_A+\sqrt{M_A(M_A+2S)}} \right)^2, \!\!&\text{if } D < D_+ \\
%     %         \frac{M_A}{2(qM_B-S)}, &\text{if } D \geq D_+
%     %     \end{cases}
%     % \end{equation}
%     % where $D := qM_B - S$ and $D_+ := \frac{M_A}{4} + \sqrt{(\frac{M_A}{4})^2 + \frac{SM_A}{2}}$.}
    
%     The proof is finalized by substituting $M_A = X_A - cS$ into the conditions derived for Cases 1 and 2. The $S_\pm$ are values for $S$ where the equilibrium solution switches between Case 1 and Case 2. They are derived from the equation $M_A = \frac{2(qM_B-S)^2}{S + (qM_B-S)}$. The condition (iii) is the condition where $S_\pm$ has an imaginary part, for which the Case 2 solution holds for all $S \in [0,X_A/c]$.
% \end{proof}

% The next lemma identifies structural properties for the function in the expression \eqref{eq:piA2_cost}, which we denote as $\pi_A^{(1)}(S)$.
% \begin{lemma}\label{lem:piA2_properties}
%     Consider the function $\pi_A^{(1)}(S)$ given by \eqref{eq:piA2_cost} for $S \in [0,X_A/c]$, and suppose $c < 1$. It has a unique critical point at $S_c := \frac{X_A}{c}(1 - \frac{c}{2-c}) \in (0,X_A/c)$. It is strictly increasing on $(0,S_c)$ and strictly decreasing on $(S_c,X_A/c)$.
% \end{lemma}
% \begin{proof}
%     To prove the first part, we show that the derivative of $\pi_A^{(1)}$ has a unique zero in $(0,M/c)$. The derivative can be written as
%     \begin{equation}
%         \frac{\partial \pi_A^{(1)}}{\partial S} = -\frac{WqM_B}{2}\frac{(f+g)((c-2)f + cg)}{fg(fg+f^2+S)^2}
%     \end{equation}
%     where $f := \sqrt{X_A-cS}$ and $g := \sqrt{X_A+(2-c)S}$. For any $S \in (0,X_A/c)$, $f,g > 0$. We thus have $\frac{\partial \pi_A^{(1)}}{\partial S} = 0$ if and only if $(2-c)f = cg$. This is equivalent to $S = S_c$.
    
%     Suppose $\pi_A^{(1)}$ is not increasing for some $S' \in (0,S_c)$, i.e. $\frac{\partial \pi_A^{(1)}}{\partial S}(S') < 0$. Observe that $\lim_{S \downarrow 0} \frac{\partial \pi_A^{(1)}}{\partial S}(S) = \frac{qM_B(1-c)}{2X_A^2} > 0$, so there must exist a $0 < S'' < S'$ for which $\frac{\partial \pi_A^{(1)}}{\partial S}(S'') = 0$. However, this contradicts the fact that $S_c$ is the unique critical point in $(0,X_A/c)$.
    
%     By similar arguments as above, we can establish that $\pi_A^{(1)}$ is strictly decreasing on $S \in (S_c,X_A/c)$. In particular, we observe that $\lim_{S \uparrow X_A/c} \frac{\partial \pi_A^{(1)}}{\partial S}(S)  < 0$.
% \end{proof}

% We are now ready to prove the main theorem. We will denote the function in the expression \eqref{eq:piA3_cost} as $\pi_A^{(2)}(S)$.
% \begin{proof}[Proof of Theorem \ref{thm:investment}]
%     % The unique critical point of $\pi_A^{(2)}$ is calculated to be $P_c := \frac{M}{c}(1 - \frac{c}{2-c})$. The function $\pi_A^{(2)}$ is strictly increasing on $P \in [0,P_c)$ and strictly decreasing on $P \in (P_c,M/c]$.
    
%     Let us suppose $c > \frac{X_A}{qM_B}$. The function $\pi_A^{(2)}$ is strictly decreasing in $S \in [0,X_A/c]$. If we assume that $X_A \leq 2qM_B(2-c)(\sqrt{1 + \frac{c}{2-c}}-1)$, then $\pi_A = \pi_A^{(2)}$ for all $S \in [0,M/c]$ (Lemma \ref{lem:piA_unif_cost}). Consequently, $S^* = 0$. We then assume $2(2-c)qM_B(\sqrt{1 + \frac{c}{2-c}}-1) < X_A < cqM_B$. We claim that there are no critical points in the interval $S \in [0,X_A/c]$. This boils down to showing $S_c < S_-$, which can be written as 
%     \begin{equation}\label{eq:thmProof_inequality}
%         \begin{aligned}
%             \frac{X_A}{c}-qM_B &< \frac{X_A}{2(2-c)} - \\
%             &\quad\sqrt{\frac{qM_B(X_A-cqM_B)}{2-c} + \left(\frac{X_A}{2(2-c)} \right)^2}
%         \end{aligned}
%     \end{equation}
%     This holds, since the LHS above is negative and the RHS above is positive. Using Lemma \ref{lem:piA2_properties}, we deduce that $\pi_A$ must be a strictly decreasing function in $S \in [0,X_A/c]$. Consequently, $S^* = 0$.
    
%     Now, let us suppose $c < \frac{X_A}{qM_B}$. The function $\pi_A^{(1)}$ is strictly increasing in $P \in [0,X_A/c]$. If $S_- > 0$, then from Lemma \ref{lem:piA_unif_cost}, $\pi_A = \pi_A^{(1)}$ for $S \in [0,S_-]$ and $\pi_A = \pi_A^{(1)}$ for $S \in (S_-,X_A/c]$. We claim the maximal value of $\pi_A$ is attained at $S_c$, i.e. $S^* = S_c$. This is equivalent to showing that $S_c > S_-$, i.e. the opposite inequality of \eqref{eq:thmProof_inequality}. This always holds, since the LHS in \eqref{eq:thmProof_inequality} is positive and the RHS is negative.
    
%     If $S_- \leq 0$, then from Lemma \ref{lem:piA_unif_cost}, $\pi_A = \pi_A^{(1)}$ for all $S \in [0,X_A/c]$ and thus $S^* = S_c$. 
    
% \end{proof}

% % % % % % % % % % % % % % % %
% % % % % % % % % % % % % % % %
% % % % % % % % % % % % % % % %
